# Supplementary material for: Learning Human-to-Robot Handovers from Point Clouds
Source: arXiv:2303.17592 source file (2023-03-30)
Supplement: Supplementary file 2 [file 05_glossary.tex]

\section{Glossary}
\label{app_glossary}
